# Supplementary material for: Rebooting ACGAN: Auxiliary Classifier GANs with Stable Training
Source: arXiv:2111.01118 source file (2021-11-01)
Supplement: Supplementary file 1 [file Table_Mog.tex]

\begin{table}[h!]
\centering
\caption{Top 1 and Top 5 ImageNet classification accuracies on images sampled from ACGAN~\cite{Odena2017ConditionalIS}, BigGAN~\cite{Brock2019LargeSG}, ContraGAN~\cite{kang2020contragan}, and ReACGAN~(ours). We use ImageNet pre-trained Inception-V3 model~\cite{Szegedy2016RethinkingTI}. To sample images from GANs, we use the best checkpoints during 200k generator training.} 
\vspace{2mm}
  \resizebox{0.95\textwidth}{!}{
\begin{tabular}{lccccc}
\cmidrule[1.0pt]{1-6}
 & Real data~(validation) & ACGAN~\cite{Odena2017ConditionalIS} & BigGAN~\cite{Brock2019LargeSG} & ContraGAN~\cite{kang2020contragan} & ReACGAN \\
\cmidrule[1.0pt]{1-6}
Distance of class 0 & 70.822 & 62.412 & 29.994 & 2.866 &  23.210\\
Top-5 Accuracy (\%) & 89.574 & 84.899 & 53.842 & 11.482 & 51.602\\
\cmidrule[1.0pt]{1-6}
IS~\cite{Salimans2016ImprovedTF}$\uparrow$ & 173.33 & 62.99 & 28.63 & 25.25 & 50.30\\
FID~\cite{Heusel2017GANsTB}$\downarrow$ & - & 26.35 & 24.68 & 25.16 & 16.32 \\
\cmidrule[1.0pt]{1-6}
\end{tabular}}
\label{table:mog}
\end{table}
